# Supplementary material for: Particle Filtering for Large Dimensional State Spaces with Multimodal Observation Likelihoods
Source: arXiv:0805.0053 source file (2008-05-01)
Supplement: Supplementary file 1 [file appendix.tex]

\section*{Appendix}

%{\bf Proof of Theorem \ref{unimodthm}: }
%\\
%\\
%
%
%
{\bf Proof of Theorem \ref{ismtthm}: }
From  (\ref{defsigis}) and (\ref{defL}), we have
\beq
(\Sigma_{IS}^i)^{-1} = (\nabla_{X_{t,r}}^2 L^i) (m_t^i) = (\nabla_{X_{t,r}}^2 E) (X_{t,s}^i, m_t^i) + \Sigma_r^{-1} \ \ \
\eeq
By Theorem \ref{unimodthm}, $m_t^i$ is the unique minimizer of $L^i$ and it lies inside $\R_{LC}$. Inside $\R_{LC}$, $E$ is convex, i.e. $(\nabla_{X_{t,r}}^2 E) (X_{t,s}^i, m_t^i) \ge 0$. Thus $(\Sigma_{IS}^i)^{-1} \ge \Sigma_r^{-1}$ or equivalently $\Sigma_{IS}^i \le \Sigma_r$. This implies that
\bea
\trace(\Sigma_{IS}^i) \le \trace(\Sigma_r)
\label{smaller}
\eea
Note that $m_{t}^i$ is a function of $\Sigma_r$ and of $X_{t-1:t,s}^i$, $Y_t$ and  $X_{t-1,r}^i=m_{t-1}^i$. $m_{t-1}^i$ is itself a function of $\Sigma_r$ and of $X_{t-2:t-1,s}^i$, $Y_{t-1}$ and $X_{t-2,r}^i = m_{t-2}^i$ and so on. Thus, $m_{t}^i$ is a function of $\Sigma_r$, $X_{1:t,s}^i, Y_{1:t}$.
For any value of $X_{1:t,s}^i, Y_{1:t}$, and  $\forall \eps_1 > 0$, we have
\bea
\ds
Pr(||X_{t,r} - m_t^{i}|| > \eps_1)   \sle  \sum_{p=1}^{M_r} Pr([X_{t,r} - m_t^{i}]_p^2> \frac{\eps_1^2}{M_r} ) \nn \\
\sle \sum_{p=1}^{M_r} \frac{4(\Sigma_{IS}^i)_{p,p} }{9\eps_1^2/(M_r)} = \frac{4 M_r\trace(\Sigma_{IS}^i)}{9\eps_1^2} \nn \\
\sle \frac{4M \trace(\Sigma_r)}{9\eps_1^2}  % \frac{\sum_{p=1}^{M-K} \Delta_{p+K}(M-K)}{\eps^2} = %\defn \frac{\Delta_{tot}(M)}{\eps^2}
\label{convinprob}
\eea
The first inequality follows since $\{X_{t,r} \in \re^{M_r}: ||X_{t,r} - m_t^{i}|| > \eps_1 \} \subseteq \{X_{t,r} \in \re^{M_r}: \mbox{there exists at least one $p$ for which $([X_{t,r} - m_t^{i}]_p)^2 >  \eps_1^2/M_r$} \}$ and applying the union bound on the probability of this event.
The second inequality follows by applying Vysochanskij-Petunin inequality  \cite[Pg 137]{stats} to $([X_{t,r} - m_t^{i}]_p)$. This can be applied because $([X_{t,r} - m_t^{i}]_p)$  has a unimodal (Gaussian) pdf.
The third inequality holds because of (\ref{smaller}).
Thus Theorem \ref{ismtthm}, \ref{ismtinprob}) follows.
%From (\ref{convinprob}), for any $\eps_1, \eps_2 > 0$, $Pr(||X_{t,r}^{i} - m_t^{i}|| > \eps_1) < \eps_2$ if $\trace(\Sigma_r) < \delta_{\eps_1, \eps_2} = \eps_1^2 \eps_2/M$ and this holds for any given values of $X_{1:t,s}^i, Y_{1:t}$. Thus Theorem \ref{ismtthm}.\ref{ismtinprob} follows.
% \\
Theorem \ref{ismtthm}, \ref{ismtinms}) holds since
$\E[||X_{t,r} - m_t^{i}||^2  |X_{1:t,s}^i,Y_{1:t} ] = \trace(\Sigma_{IS}^i) \le \trace(\Sigma_r)$.% This inequality holds because of (\ref{smaller}). ~~$\blacksquare$
\\
\\
\setlength{\arraycolsep}{0.005cm}
